# Supplementary material for: It's Not Easy Being Wrong: Large Language Models Struggle with Process of Elimination Reasoning
Source: arXiv:2311.07532 source file (2024-06-07)
Supplement: Supplementary file 1 [file commonsense.tex]

\begin{table*}[t]
\centering
\small
\begin{tabular}{@{}l|cccc|cccc@{}}
\toprule
\multicolumn{1}{c|}{\multirow{2}{*}{\textbf{Model}}} & \multicolumn{4}{c|}{\textbf{Commonsense QA}} & \multicolumn{4}{c}{\textbf{Social IQa}} \\
\multicolumn{1}{c|}{} & DA Base & DA COT & PoE Base & PoE COT & DA Base & DA COT & PoE Base & PoE COT \\ \midrule
LLaMA 7B & 0.816 & 0.860 & 0.320 & 0.458 & 0.762 & 0.758 & 0.440 & 0.548 \\
LLaMA 13B & 0.858 & 0.868 & 0.266 & 0.420 & 0.772 & 0.806 & 0.408 & 0.578 \\
LLaMA 70B & 0.930 & 0.914 & 0.846 & 0.808 & 0.876 & 0.844 & 0.814 & 0.796 \\ \midrule
Falcon 7B & 0.516 & 0.690 & 0.472 & 0.466 & 0.518 & 0.650 & 0.500 & 0.482 \\
Falcon 40B & 0.892 & 0.876 & 0.740 & 0.530 & 0.808 & 0.818 & 0.718 & 0.628 \\
Falcon 180B & 0.924 & 0.922 & 0.912 & 0.786 & 0.858 & 0.840 & 0.802 & 0.716 \\ \midrule
GPT 3.5 & 0.888 & 0.926 & 0.778 & 0.848 & 0.838 & 0.858 & 0.820 & 0.748 \\ \bottomrule
\end{tabular}
\caption{\label{table:commonsense_eval}Evaluation of Direct Answer (DA) and Process of Elimination (PoE) strategies on commonsense reasoning datasets, with and without chain-of-thought reasoning.}
\end{table*}
