# Supplementary material for: It's Not Easy Being Wrong: Large Language Models Struggle with Process of Elimination Reasoning
Source: arXiv:2311.07532 source file (2024-06-07)
Supplement: Supplementary file 2 [file science.tex]

\begin{table*}[t]
\centering
\small
\begin{tabular}{@{}l|cccc|cccc@{}}
\toprule
\multicolumn{1}{c|}{\multirow{2}{*}{\textbf{Model}}} & \multicolumn{4}{c|}{\textbf{ARC}} & \multicolumn{4}{c}{\textbf{OpenBookQA}} \\
\multicolumn{1}{c|}{} & DA Base & DA COT & PoE Base & PoE COT & DA Base & DA COT & PoE Base & PoE COT \\ \midrule
LLaMA 7B & 0.770 & 0.784 & 0.478 & 0.494 & 0.790 & 0.850 & 0.399 & 0.593 \\
LLaMA 13B & 0.816 & 0.830 & 0.266 & 0.578 & 0.818 & 0.856 & 0.277 & 0.529 \\
LLaMA 70B & 0.930 & 0.930 & 0.744 & 0.874 & 0.938 & 0.922 & 0.677 & 0.824 \\ \midrule
Falcon 7B & 0.544 & 0.544 & 0.470 & 0.420 & 0.523 & 0.629 & 0.483 & 0.453 \\
Falcon 40B & 0.836 & 0.804 & 0.656 & 0.542 & 0.848 & 0.868 & 0.747 & 0.683 \\
Falcon 180B & 0.938 & 0.888 & 0.874 & 0.814 & 0.924 & 0.928 & 0.888 & 0.812 \\ \midrule
GPT 3.5 & 0.914 & 0.946 & 0.856 & 0.852 & 0.892 & 0.908 & 0.745 & 0.850 \\ \bottomrule
\end{tabular}
\caption{\label{table:science_eval}Evaluation of Direct Answer (DA) and Process of Elimination (PoE) strategies on scientific reasoning datasets, with and without chain-of-thought reasoning.}
\end{table*}
